# Supplementary material for: Touch2Shape: Touch-Conditioned 3D Diffusion for Shape Exploration and Reconstruction
Source: arXiv:2505.13091 source file (2025-05-19)
Supplement: Supplementary file 1 [file fig_network_suppl.tex]

%------------------------------------------------------------------------
\begin{figure*}[htbp]
  \centering
  \includegraphics[width=0.999\linewidth]{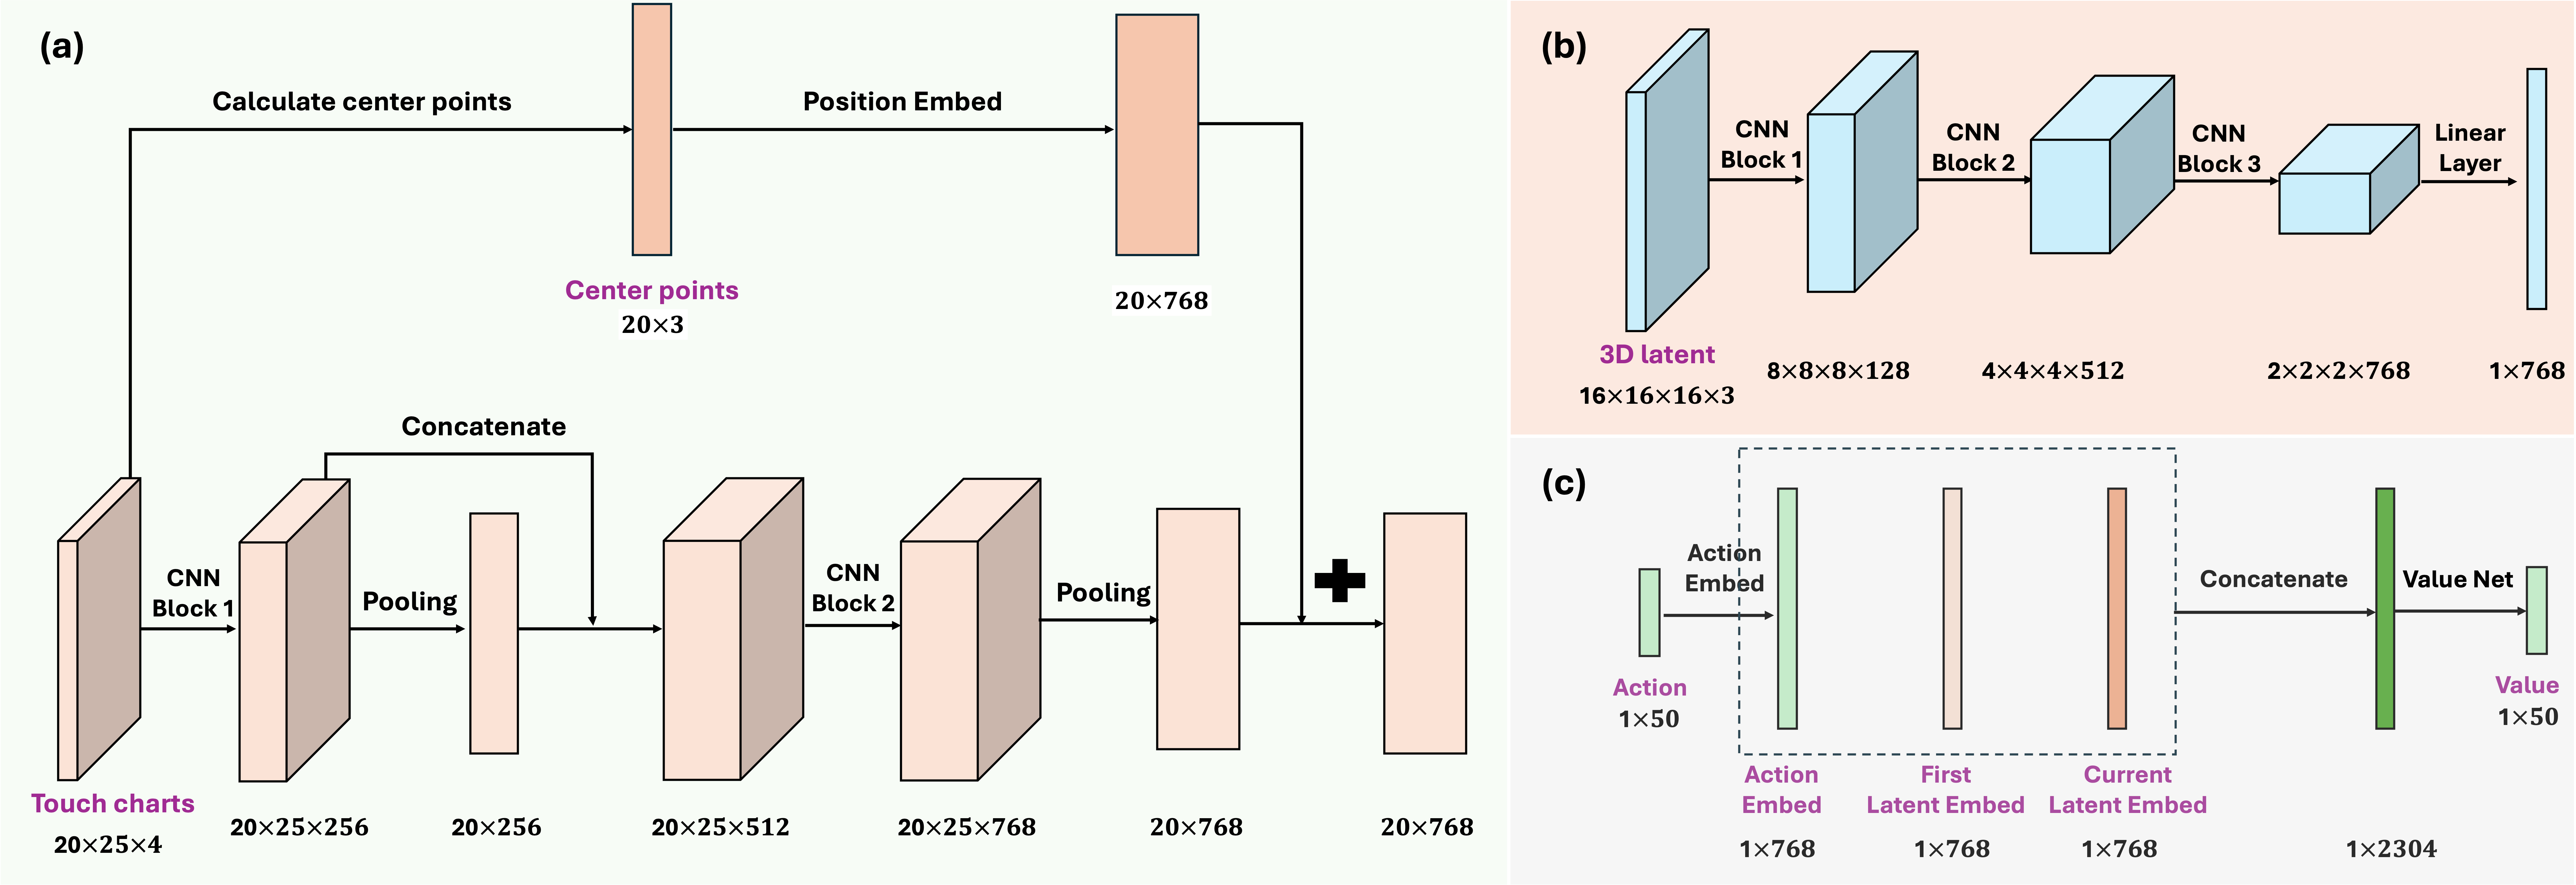}
  \caption{\label{fig:fig_network_suppl}
         The network architectures of (a) the touch embedding module, (b) the latent encoder and (c) the policy model.
         }
\vspace{-0.4cm} 
\end{figure*}
